# Supplementary material for: RoadAtlas: Intelligent Platform for Automated Road Defect Detection and Asset Management
Source: arXiv:2109.03385 ancillary file (2021-09-09)
Supplement: Supplementary file 1 [file RoadAtals_Demonstration_Slides.pdf]

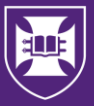

THE UNIVERSITY  
OF QUEENSLAND  
AUSTRALIA

CREATE CHANGE

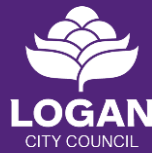

# RoadAtlas: Intelligent Platform for Automated Road Defect Detection and Asset Management

Zhuoxiao Chen<sup>1</sup>, Yiyun Zhang<sup>1</sup>, Yadan Luo<sup>1</sup>, Zijian Wang<sup>1</sup>, Jinjiang Zhong<sup>2</sup>, Anthony Southon<sup>2</sup>

{zhuoxiao.chen, yiyun.zhang, y.luo, zijian.wang}@uq.edu.au,

{JinjiangZhong, AnthonySouthon}@logan.qld.gov.au

<sup>1</sup>The University of Queensland, <sup>2</sup>Logan City Council, Australia

# Introduction

## Motivation

- Local government needs to employ manual road surveys to monitor road damages to cracks and markings.
- Requires well-trained inspectors to review the collected street images to identify and locate the cracks and road markings.
- This is a costly and time-consuming procedure (around \$350K to \$400K per survey).
- It prevents local government from conducting frequent surveys to keep the data up to date.
- It not only affects the aesthetic value of the city, but also increases risks of injury and fatality faced by pedestrians.

## Objective

- Develop a novel AI-powered road defects and assets management platform – RoadAtlas.
- It can automatically detect road defects and road markings at pixel level precision.
- It can support automatically demonstrate and report types, severity, location and evidence of road anomalies for planning the follow-up repairs.

# Overall Framework of RoadAtlas

- Dashboard: provides functions such as performing recognition, uploading images, exporting results, etc.
- Deep Models:
  - Road defect recognition by a crack detector and a crack segmenter.
  - Road marking parsing by a crack segmenter.
- Backend:
  - APIs developed with Python Flask to process data, queries and procedure.
  - MongoDB and hard disk storage for data management and maintenance.

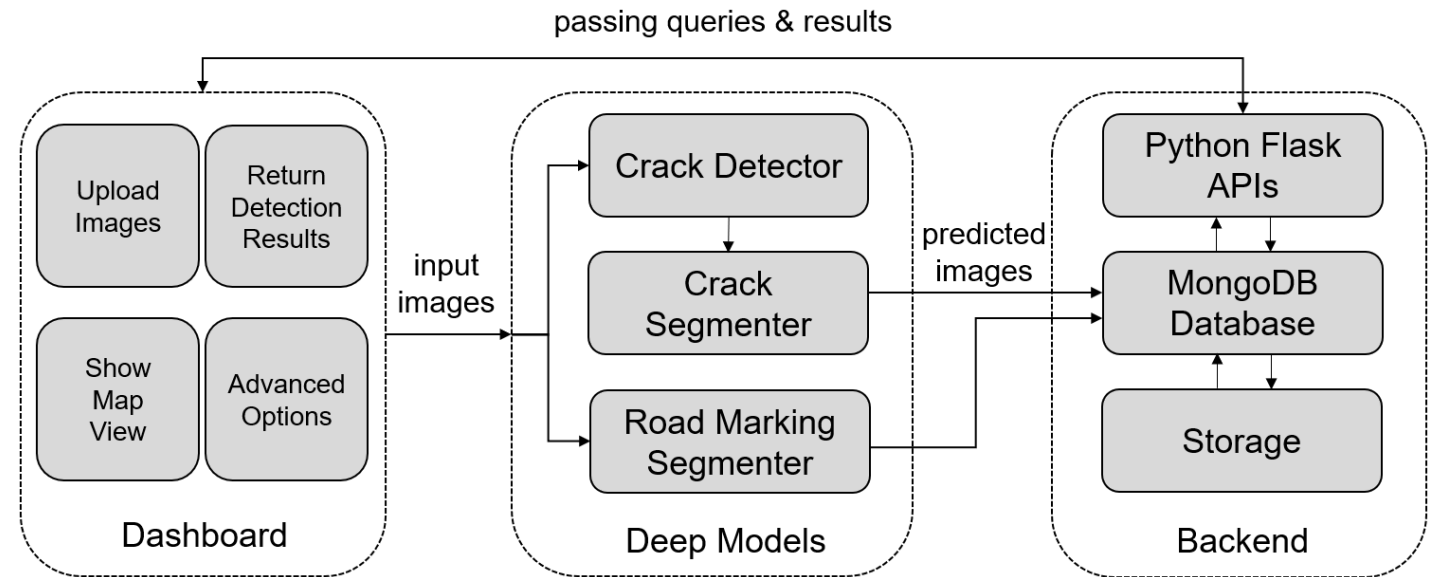

# Dashboard & Backend

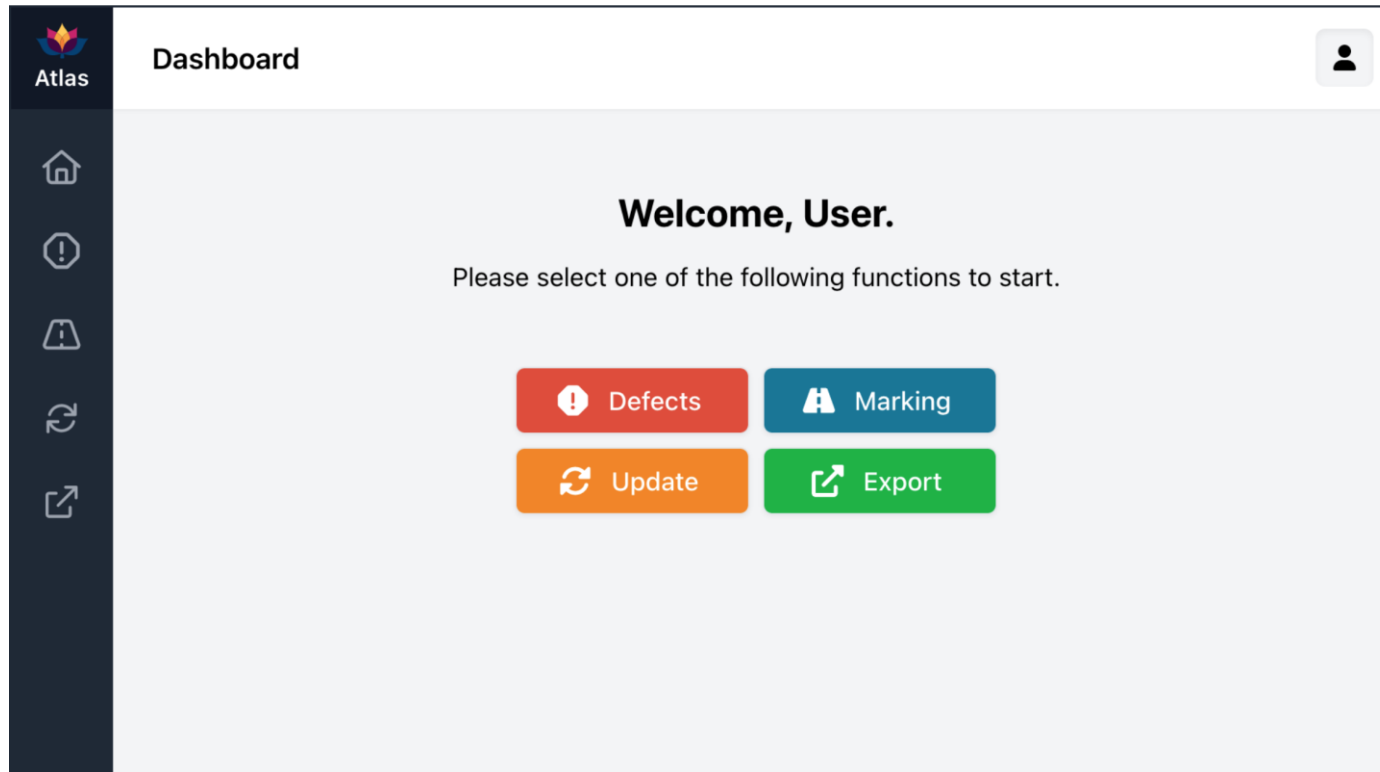

## Frontend

- Road Defect & Road Marking: allow users to inspect and validate labelled images from the database.
- Database Update: upload unprocessed images to the deep model for defect and marking detection.
- Report Export: save validated images data as CSV or JSON-formatted

## Backend

- All the functions are processed by calling APIs developed with Python Flask.
- All data are stored in well-structured MongoDB for fast retrieval and insertion

# Dashboard & Backend

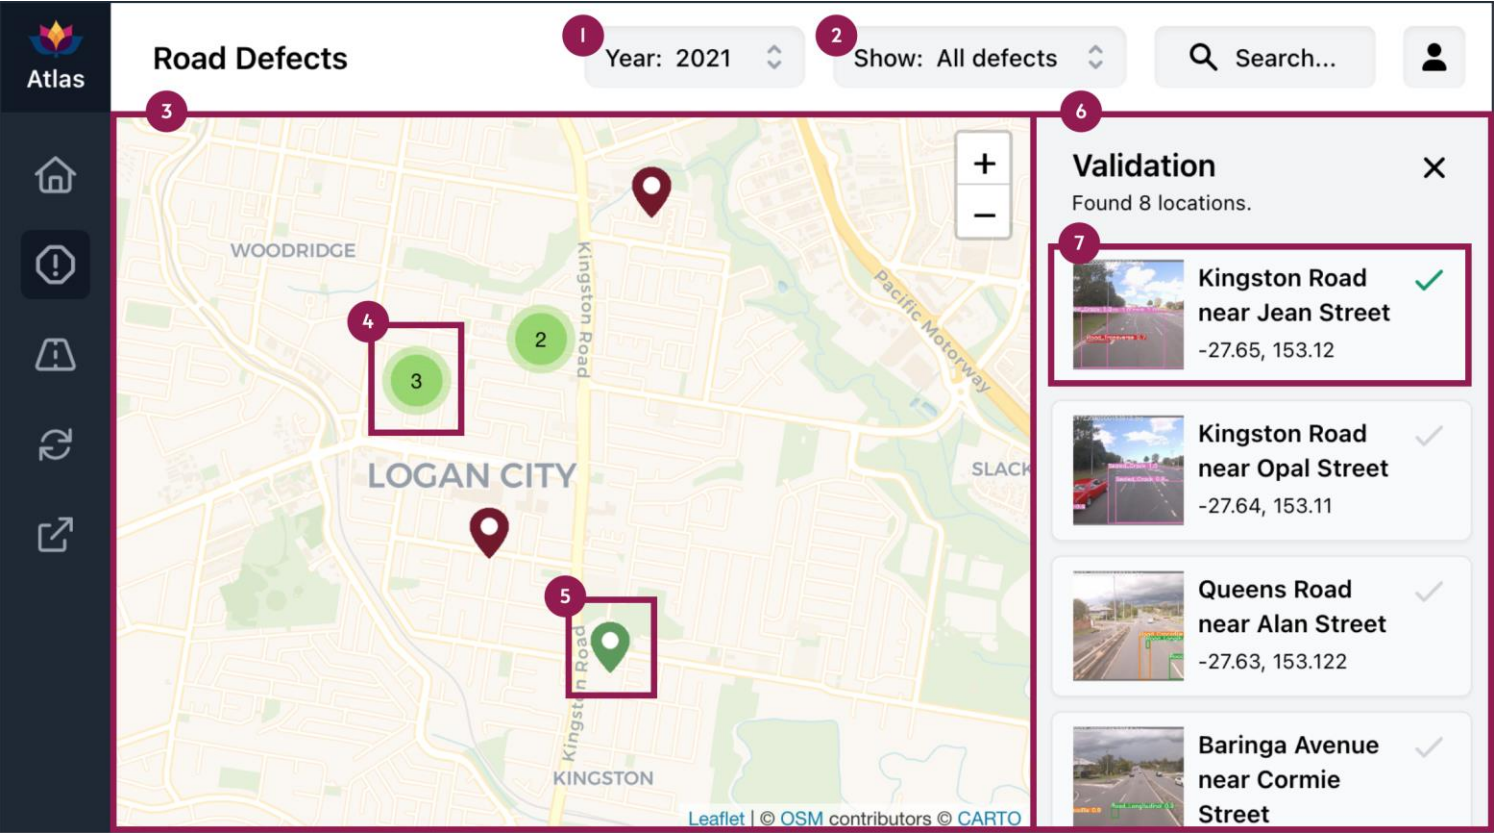

| # | Name                 | Description                                                                                                                                                                                                                                                                                                                              |
|---|----------------------|------------------------------------------------------------------------------------------------------------------------------------------------------------------------------------------------------------------------------------------------------------------------------------------------------------------------------------------|
| 1 | Data Range Selection | Selects the year range of data showing.                                                                                                                                                                                                                                                                                                  |
| 2 | Data Filter          | Filters data shown in the map view by defect type (e.g. potholes or maintenance related defects).                                                                                                                                                                                                                                        |
| 3 | Map View             | Shows the map of the Logan city and map pins.                                                                                                                                                                                                                                                                                            |
| 4 | Cluster Pin          | Represents the number of data in the nearby area.                                                                                                                                                                                                                                                                                        |
| 5 | Defect Pin           | Represents a detected defect in this place.                                                                                                                                                                                                                                                                                              |
| 6 | Validation Panel     | Provides details of the data (e.g. road cracks) in the selected area for user to view and validate.                                                                                                                                                                                                                                      |
| 7 | Data Detail          | Shows the details of an individual piece of data (e.g. a single road crack). It will display the coordinates, estimated street names, images and unique IDs of the data. When the user clicks on the detail, they can see a detailed screen and validate the data manually (e.g. mark the road cracking data as fixed, or not an issue). |

# Road Defect Recognition – Data Annotation

- We employed 5 annotators to label 10K Images with pixel-level polygons.
- We consider 8 classes including *\_background\_*, *Kerb\_Cracking*, *Road\_Crocodile*, *Road\_Longitudinal*, *Road\_Transverse*, *Road\_Block* and *Sealed\_Crack*.

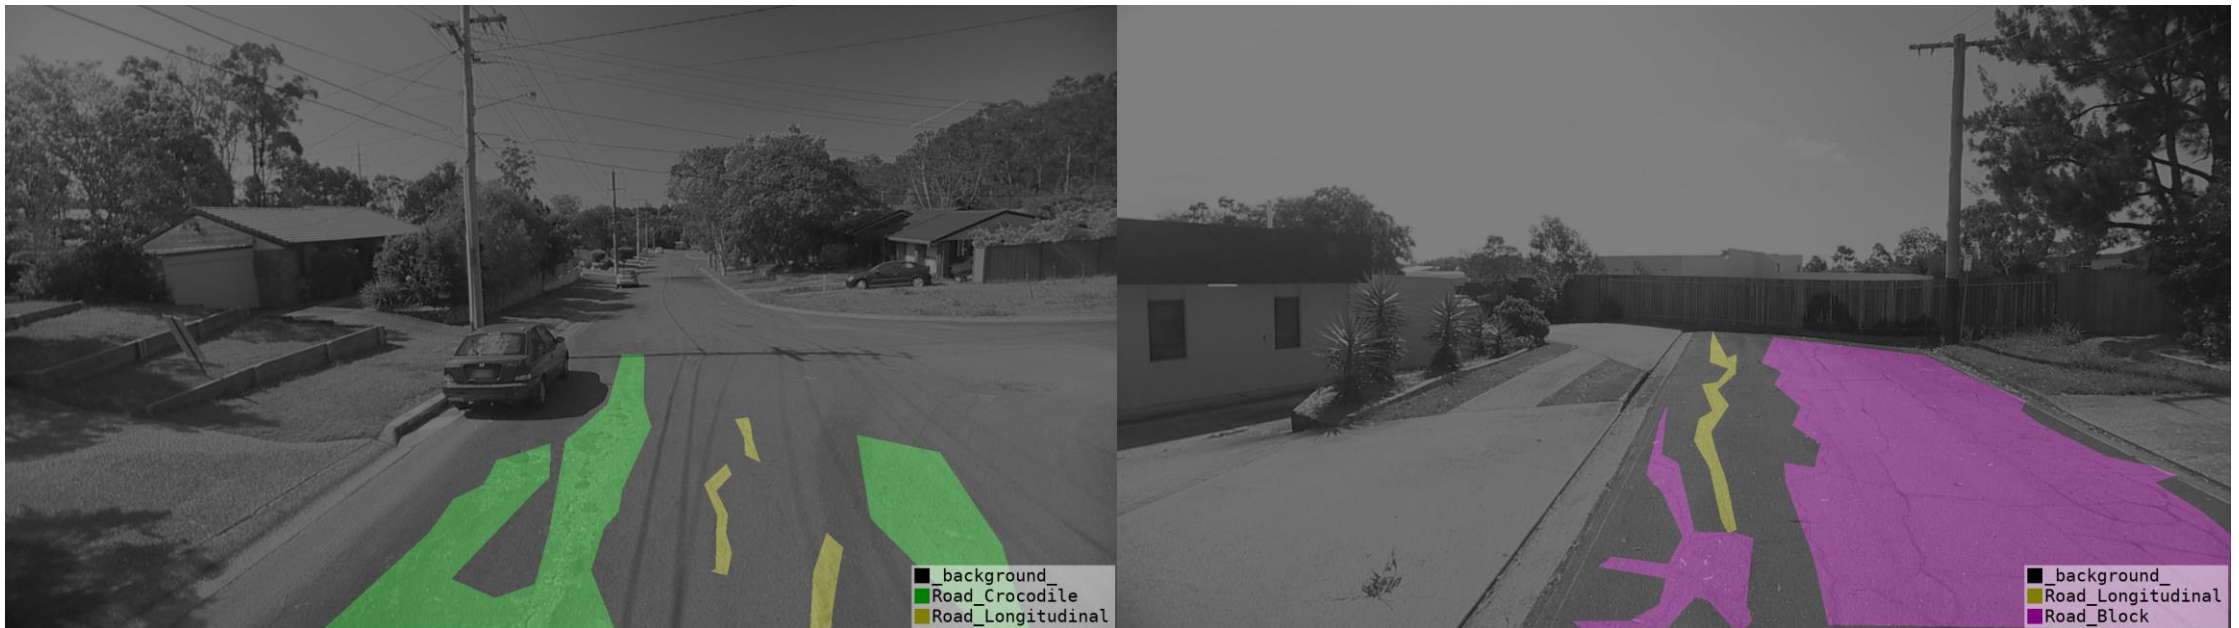



# Road Defect Recognition – Deep Models

- Crack Detector [1] is trained with minimised bounding boxes covering polygon labels, to produce bounding boxes for each crack.
- Crack Segmenter [2] is trained with polygon labels, to produce pixel-level predictions for the crack inside each bounding box.
- Performance on the labelled set: *map\_0.5: **0.9724** mAP\_0.5:0.95: **0.7622** prec **0.7319** recall **0.9875***

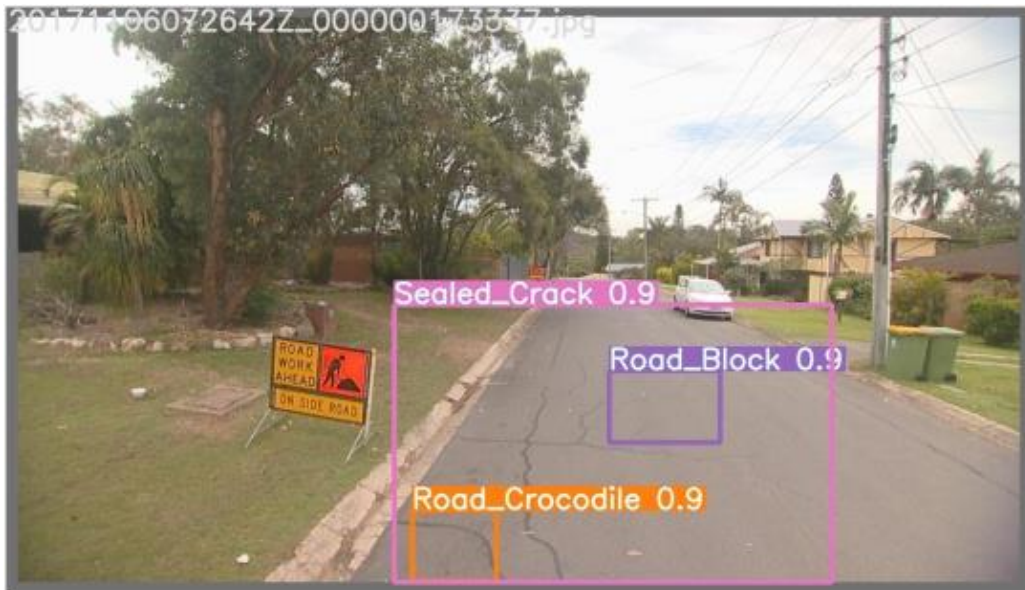

Predicted bounding boxes by Crack Detector

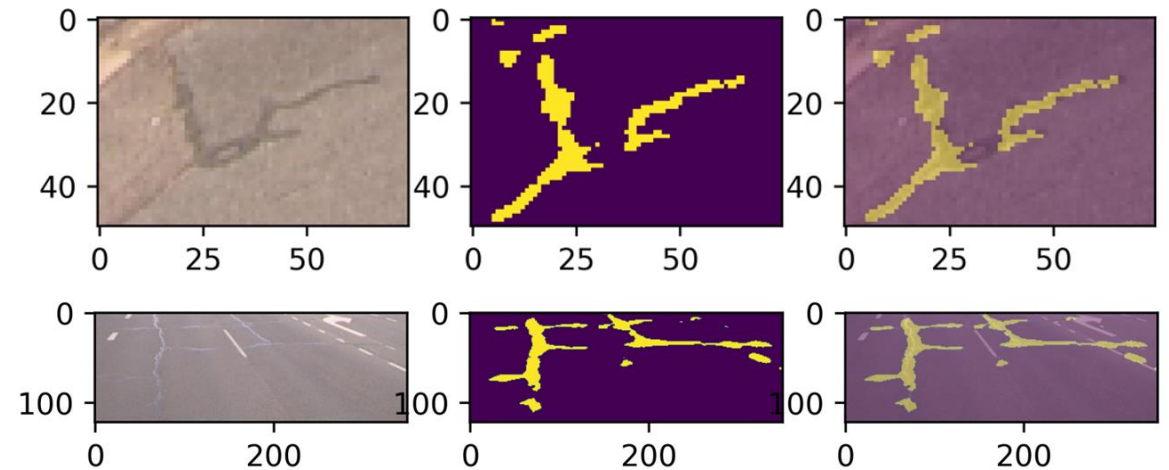

Pixel-level Predictions by Crack Segmenter

# Road Marking Parsing

## Road Marking Segmentation:

- Road Marking Segmenter [3] is trained with Apollo benchmark dataset [4], to produce pixel-level predictions for road markings.

## Refinement and Filling:

- a) Region of Interest (ROI) detection – street in our case.
- b) Low-level contour detection and Projection to bird eye view.
- c) The projected prediction map by Road Marking Segmenter.

We compare (b) and (c) to fill in low-level contours if two objects are highly overlapped.

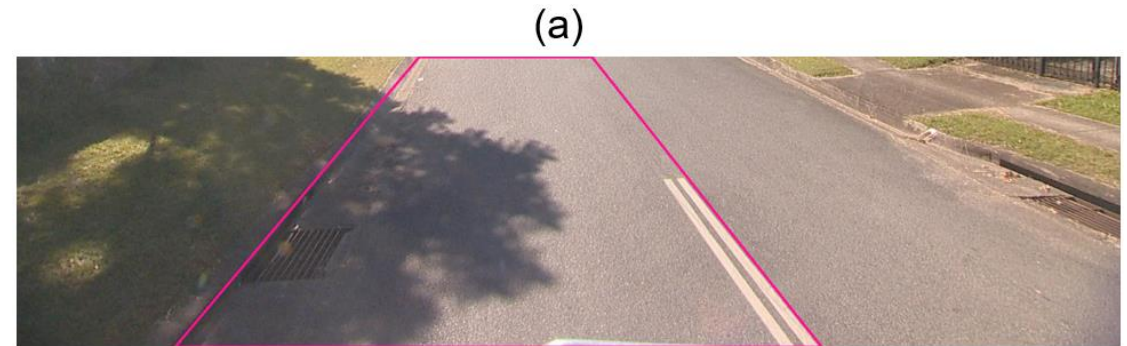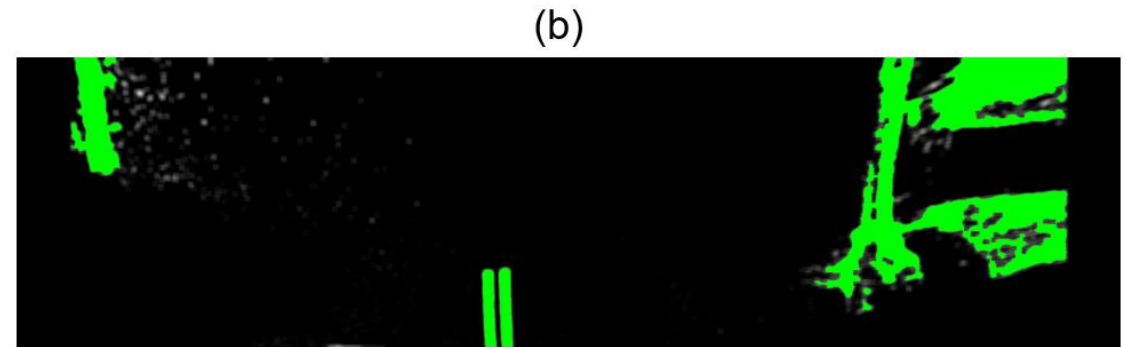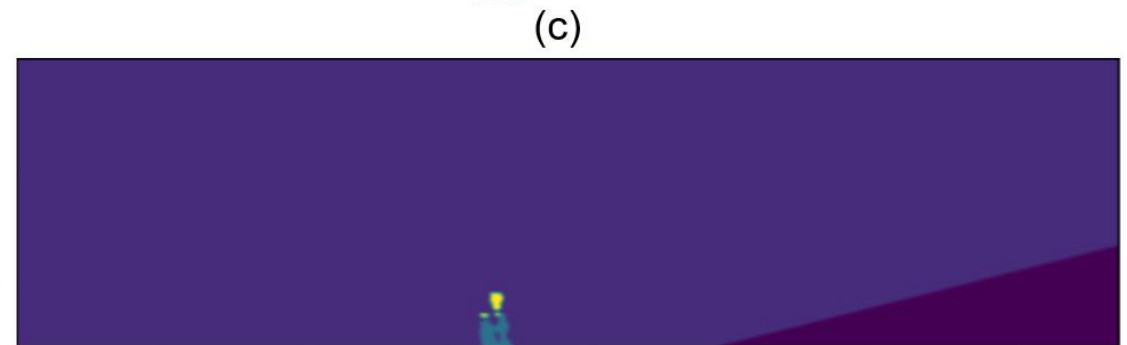



# Road Marking Parsing

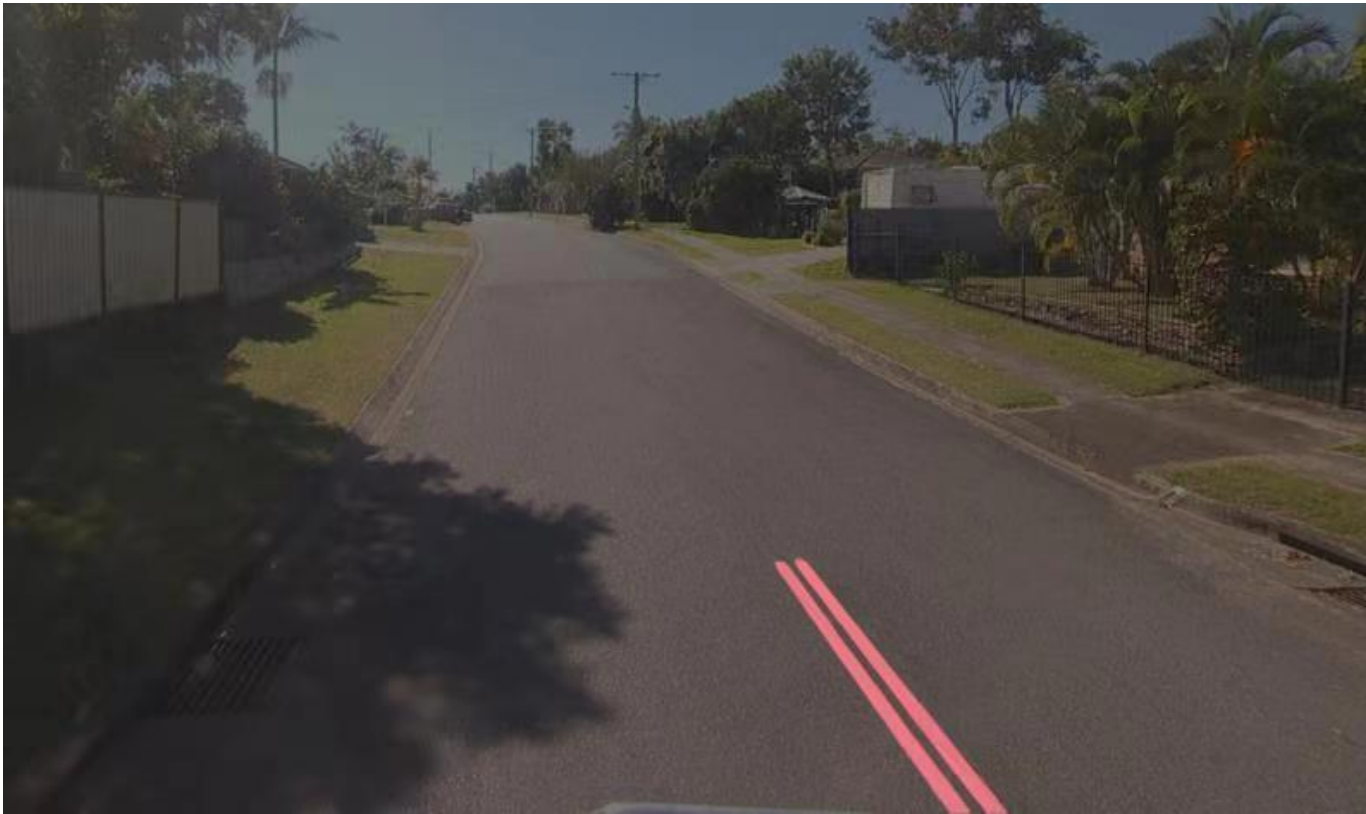

Refined Predictions for road marking

| Type           | Colour | Use                    |
|----------------|--------|------------------------|
| solid          | w      | dividing               |
| solid          | y      | dividing               |
| double solid   | w/y    | dividing, no pass      |
| solid & broken | w/y    | dividing, one-way pass |
| broken         | w/y    | guiding                |
| double broken  | y      | guiding                |
| solid          | w      | stopping               |
| solid          | w/y    | chevron                |
| solid          | w      | parking                |
| crosswalk      | w      | zebra                  |
| arrow          | w      | u-turn                 |
| arrow          | w      | thru                   |
| arrow          | w      | thru & left turn       |
| arrow          | w      | thru & right turn      |
| arrow          | w      | left turn              |
| arrow          | w      | right turn             |
| arrow          | w      | left & right turn      |
| arrow          | w      | left & u-turn          |
| bump           | n/a    | speed reduction        |
| diamond        | w/y    | zebra attention        |
| rectangle      | w/y    | no parking             |

Roadmarks labels considered in our system

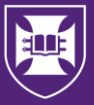

# THANKS!

Do you have any questions?

[zhuoxiao.chen@uq.edu.au](mailto:zhuoxiao.chen@uq.edu.au)

[uqyluo@uq.edu.au](mailto:uqyluo@uq.edu.au)

The University of Queensland

## Reference

- [1] Glenn Jocher. 2020.ultralytics/yolov5: v3.1 - Bug Fixes and Performance Improvements. <https://doi.org/10.5281/zenodo.4154370>
- [2] Zhao, H., Shi, J., Qi, X., Wang, X., & Jia, J. (2017). Pyramid scene parsing network. In *Proceedings of the IEEE conference on computer vision and pattern recognition* (pp. 2881-2890).
- [3] Ronneberger, O., Fischer, P., & Brox, T. (2015, October). U-net: Convolutional networks for biomedical image segmentation. In *International Conference on Medical image computing and computer-assisted intervention* (pp. 234-241). Springer, Cham.
- [4] Huang, X., Wang, P., Cheng, X., Zhou, D., Geng, Q., & Yang, R. (2019). The apolloscape open dataset for autonomous driving and its application. *IEEE transactions on pattern analysis and machine intelligence*, 42(10), 2702-2719.
